# Supplementary material for: The ATLAS Readout System for LHC Runs 2 and 3
Source: arXiv:2307.11557 source file (2023-07-21)
Supplement: Supplementary file 1 [file appendix.tex]

\appendix
\section{Appendix}
\label{sec:appendix}

Please always give a title also for appendices.
